# Supplementary material for: Crash-perching on vertical poles with a hugging-wing robot
Source: arXiv:2402.02092 ancillary file (2024-02-03)
Supplement: Supplementary file 1 [file Supplementary_Text.pdf]

# Supplementary Material for
*Crash-perching on vertical poles with a hugging-wing robot*

Mohammad Askari*, Michele Benciolini, Hoang-Vu Phan, William Stewart, Auke J. Ijspeert and Dario Floreano

*Corresponding author(s). E-mail(s): mohammad.askari@epfl.ch;

## This PDF file includes:

- Supplementary Fig. S1. Inertial reorientation test setup.
- Supplementary Fig. S2. Coordinate systems and state variables.
- Supplementary Fig. S3. Static model flowchart.
- Supplementary Fig. S4. Wing segmentation and configuration selection.
- Supplementary Fig. S5. Measuring friction coefficient of vertical poles.
- Legend to the Supplementary video.

# Supplementary Figures

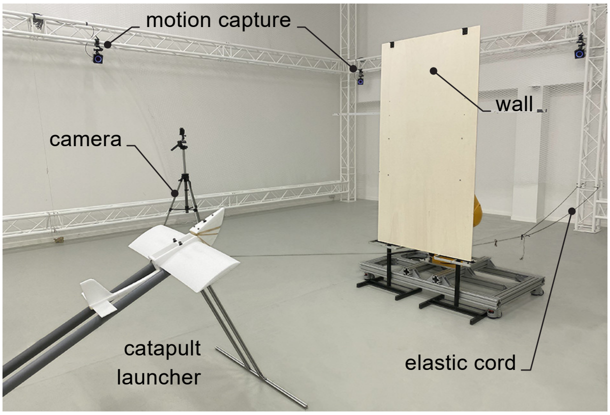


**Figure S1 Inertial reorientation test setup.** The setup consisted of a bungee-powered UAV catapult launcher with adjustable angle and speed for launching against a fixed vertical wall. High-speed videos were recorded using a camera, and OptiTrack motion capture system was used to capture trajectory data.

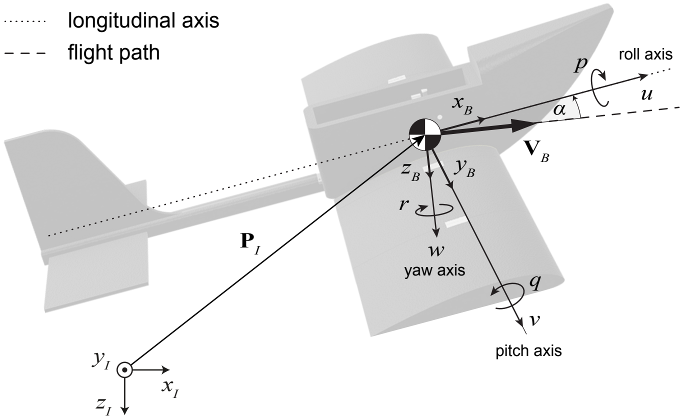


**Figure S2 Coordinate systems and state variables.** The black and white filled circle represents the center of gravity (COG). $I$ and $B$ indicate the inertial and body-attached reference frames, respectively. The 12 state variables that define the kinematics of the UAV in space are: position of the body-attached frame $\vec{\mathbf{P}}_I = [x\ y\ z]^\top$, linear velocities $\vec{\mathbf{V}}_B = [u\ v\ w]^\top$ and angular rates $\vec{\mathbf{\Omega}}_B = [p\ q\ r]^\top$ along the body-attached axes, and the body orientation based on attitude angles (roll $\phi$, pitch $\theta$, and yaw $\psi$, which are not shown for the sake of clarity). The angle of attack is indicated by $\alpha$.

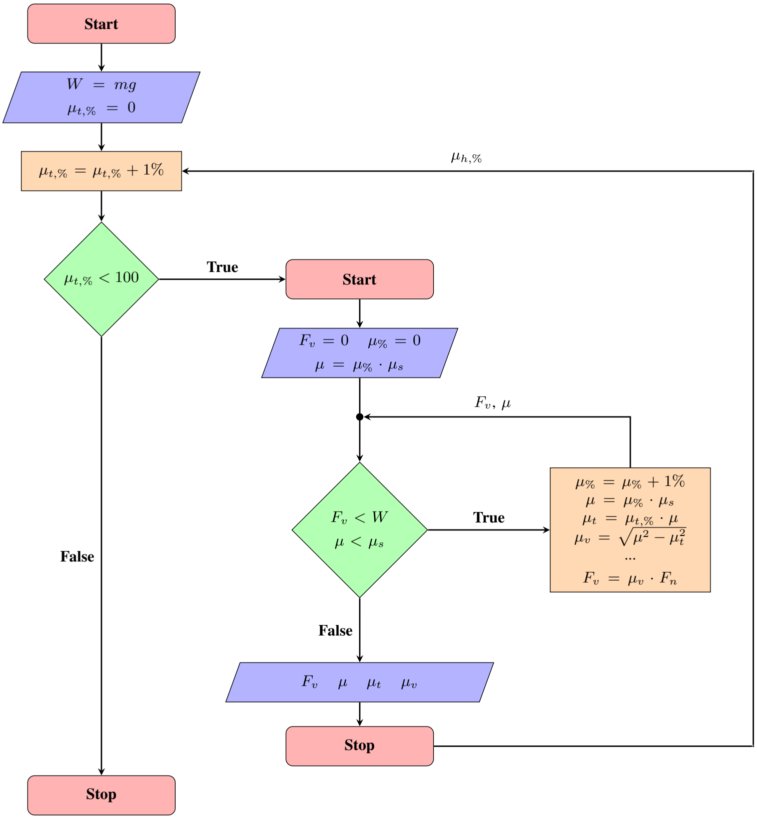


**Figure S3 Static model flowchart.** The iterative process that the model follows to find the division of friction between the horizontal and vertical directions.

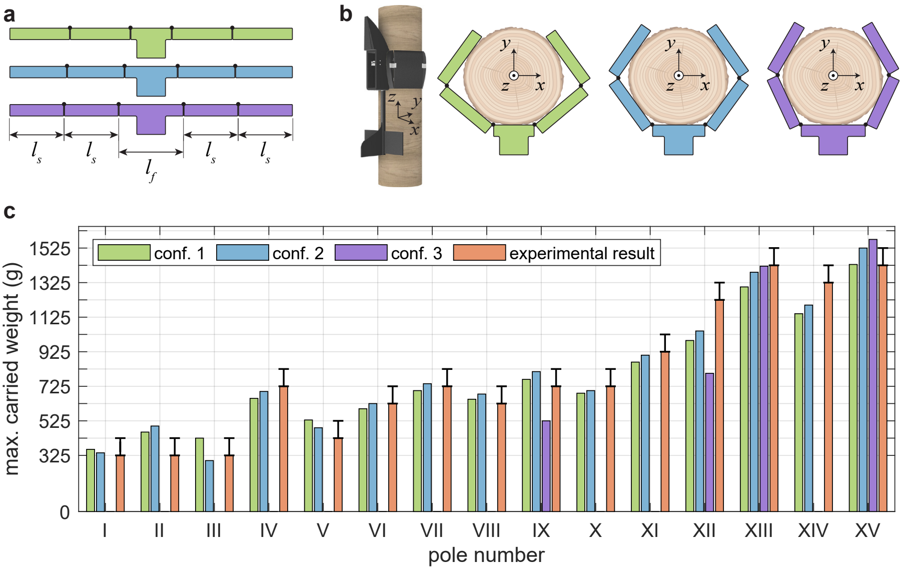


**Figure S4 Wing segmentation and configuration selection. a** Three different wing segmentation for a fixed wingspan of 960 mm, with two equally-sized folding segments per wing. These configurations are, namely, a narrow to a mid-range to a wide fuselage with respective widths of 140 mm, 180 mm, and 220 mm for the fuselage and fixed segments ($l_f$), and corresponding folding segment widths ($l_s$) of 205 mm, 195 mm, and 185 mm. **b** Top view illustration of the three wing configurations perched on a 340 mm pole. **c** Simulation results of static payload capacity for the three different wing configurations on the poles used in the static perching experiments (see Fig. 5 in the main text). The experimental data correspond to the selected wing design for PercHug, i.e., configuration 2.

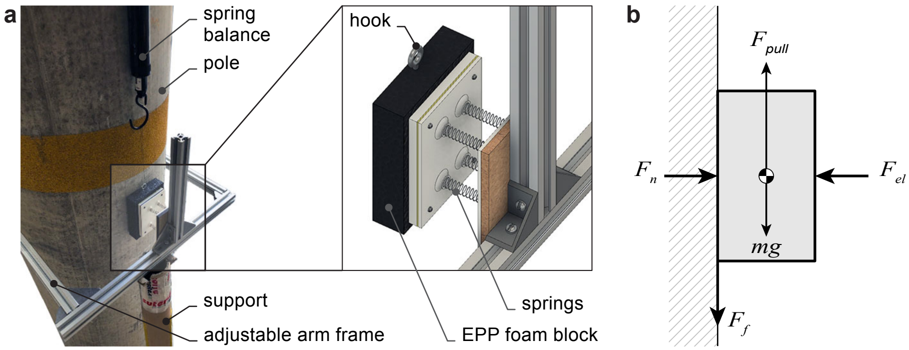


**Figure S5 Measuring friction coefficient of vertical poles. a** A photo and a close-up computer-aided design (CAD) view of the friction coefficient measuring tool used on a concrete pole. **c** Side view free body diagram of the EPP foam block representing the method employed for estimating the static friction coefficient.

## Supplementary Video

The supplementary video shows the robot design and operation of our proposed perching strategy for crash-landing winged robots on vertical poles and trees. It presents the operating principle of the method, followed by multiple successful and unsuccessful perching experiments with PercHug on trees.

Video credits: Photos by Smith, S. R. and Mattheis, S., and music by bensound.com.
